# Supplementary material for: First measurement of time-dependent CP violation in Bs -> K+K- decays
Source: arXiv:1308.1428 source file (2013-11-18)
Supplement: Supplementary file 2 [file supplementary-app.tex]

\clearpage

\section{Supplementary material}
\label{sec:Supplementary-App}

This appendix includes supplementary material that will be 
  part of the draft during the review phase but will not appear in the
  final version of the paper. Instead it will be posted as supplementary
  material alongside the paper on CDS.

\begin{figure}[!htb]
  \begin{center}
    \includegraphics[scale=0.65,bb=50 300 580 700,clip=true]{Roger-plot}
    \vspace*{-1.0cm}
  \end{center}
  \caption{
    \small %captions should be a little bit smaller than main text
    Comparison of our result to those from other experiments.
    Note that the style of this figure differs slightly from that of Figure~\ref{fig:example}}
  \label{fig:roger}
\end{figure}

\clearpage
